# Supplementary material for: Searching for Materials with High Refractive Index and Wide Band Gap: A First-Principles High-Throughput Study
Source: arXiv:1809.01132 ancillary file (2019-03-25)
Supplement: Supplementary file 1 [file supplemental_material.pdf]

# Searching for Materials with High Refractive Index and Wide Band Gap: A First-Principles High-Throughput Study (Supplemental Material)


Francesco Naccarato,[1,2,3] Francesco Ricci,[1] Jin Suntivich,[4,5] Geoffroy Hautier,[1] Ludger Wirtz,[2,3] and Gian-Marco Rignanese[1,3]

[1] *Institute of Condensed Matter and Nanosciences, Université Catholique de Louvain, 8 Chemin des étoiles, 1348 Louvain-la-Neuve, Belgium*

[2] *Physics and Materials Science Research Unit, University of Luxembourg, 162a avenue de la Faïencerie, L-1511 Luxembourg, Luxembourg*

[3] *European Theoretical Spectroscopy Facility (ETSF)*

[4] *Department of Materials Science and Engineering, Cornell University, Ithaca, New York 14853, USA*

[5] *Kavli Institute at Cornell for Nanoscale Science, Cornell University, Ithaca, New York 14853, USA*



(Dated: March 20, 2019)


## I. HINTS ABOUT THE RELATIONSHIP BETWEEN $\omega_g$ AND $E_g^d$

The relationship between the average optical gap $\omega_g$ and the direct band gap $E_g^d$ can formally be deduced from Eq. (A14) of the main text which only involves the JDOS $j(\omega)$. However, the form of $j(\omega)$ is often complex, which makes it impossible to solve the equation analytically.

Here, the solution is first derived for a simple model JDOS:

$$j(\omega) = \begin{cases} -\frac{6}{(2\sigma)^3}(\omega - E_g^d)\left(\omega - (E_g^d + 2\sigma)\right) & \text{for } E_g^d \leq \omega \leq E_g^d + 2\sigma \\ 0 & \text{elsewhere} \end{cases} \tag{S1}$$

This corresponds to a JDOS showing a single symmetric parabolic peak with a width $\sigma$ (see Model 1 in Fig. S1(a)). The analytic solution of Eq. (A14) of the main text for this model JDOS is given by:

$$\omega_g^3 = -\frac{4}{3}\sigma^3 \left[\ln\left(\frac{E_g^d + 2\sigma}{E_g^d}\right) - \frac{2\sigma(E_g^d + \sigma)}{E_g^d(E_g^d + 2\sigma)}\right]^{-1} \tag{S2}$$

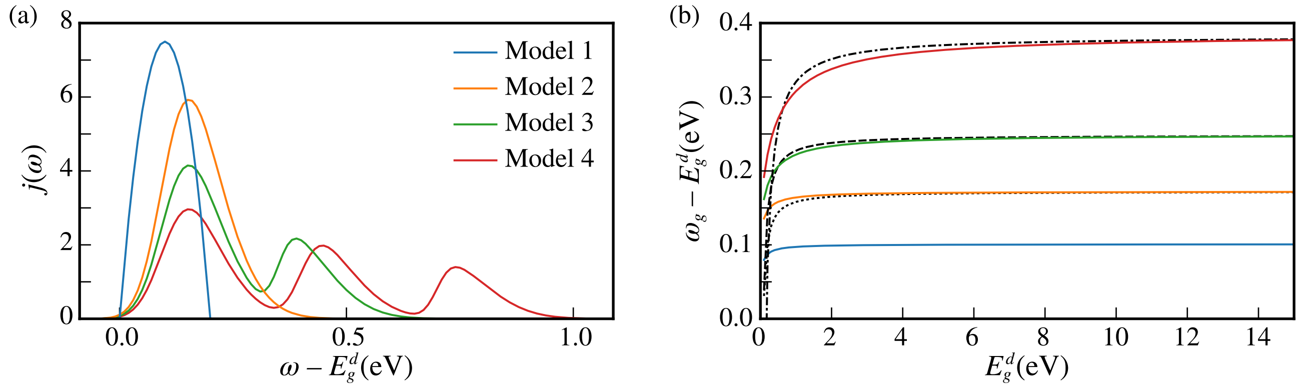


FIG. S1. (a) JDOS models (see text) and (b) corresponding relation between the average optical gap $\omega_g$ and $\omega_g$-$E_g^d$ (in eV) from Eq. (A14) of the main text. All models show the same trend which can be fitted using Eq. (S3). The results obtained by truncating the development to $n$=1 (as in Eq. (3) of the main text) are represented for Models 2, 3, and 4 using dotted, dashed, dot-dashed lines, respectively.

Using the properties of the logarithm and its Taylor expansion, we can finally write:

$$\omega_g = E_g^d + \sum_{n=0}^{\infty} \frac{c_n(\sigma)}{(E_g^d)^n} \tag{S3}$$

where the coefficients $c_n(\sigma)$ are functions of the width $\sigma$. By truncating the development to $n$=1, we find Eq. (4) of the main text.

Next, more complex JDOS models are considered. Model 2 consists of a skew normal distribution:

$$j(\omega) = \frac{A}{\sigma\sqrt{2\pi}} e^{-\frac{(\omega-\mu)^2}{2\sigma^2}} \left\{1 + \mathrm{erf}\left[\frac{\gamma(\omega-\mu)}{\sigma\sqrt{2}}\right]\right\} \tag{S4}$$

where $A$, $\mu$, $\sigma$, and $\gamma$ are the amplitude, the position, the width, and the skewness of the peak, respectively. Models 3 and 4 are obtained by summing two and three such skew normal distributions.

For all models, an analytic solution of Eq. (A14) of the main text is out of reach but $\omega_g$ can be computed numerically for different values of the peak position in order to determine its dependence with respect to $E_g^d$. In all cases, it is found that the solution has the form of Eq. (S3) and that its truncation to $n$=1 provides a good approximation (see Fig. S1(b)).

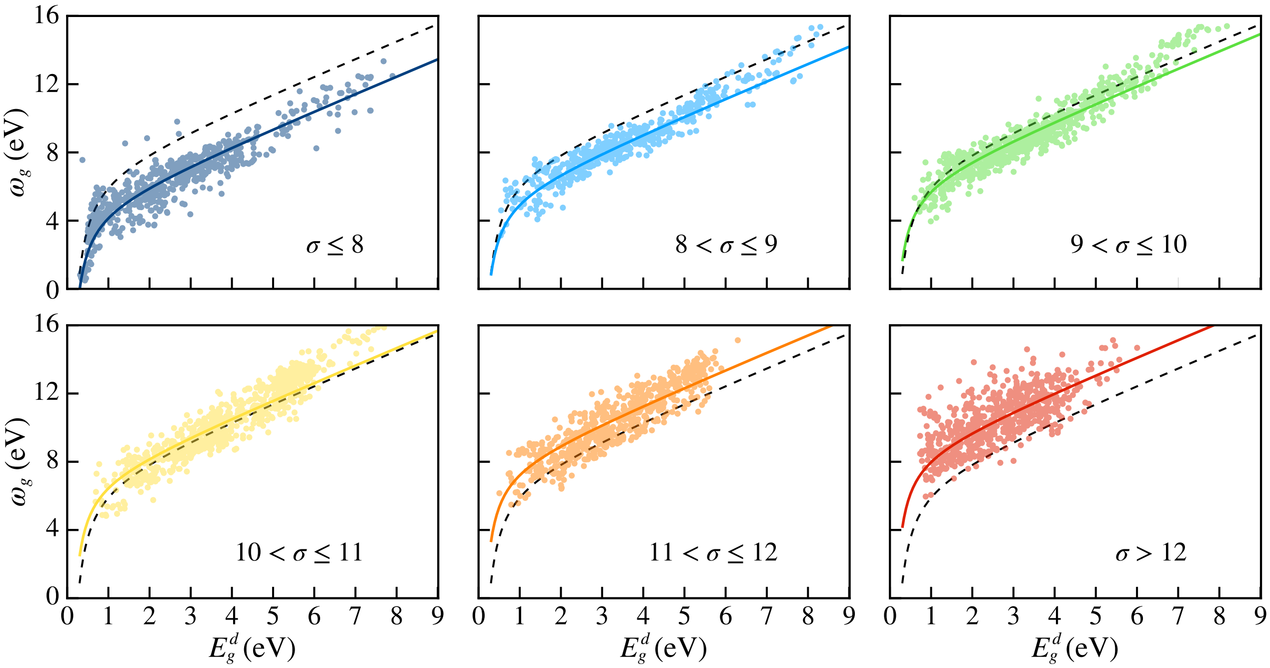


FIG. S2. Splitting of the $\omega_g$-$E_g^d$ data points considering the different ranges of the width $\sigma$. For each panel, the dashed black line corresponds to $\omega_g = E_g^d + 6.85 - 1.68/E_g^d$ which was obtained by fitting all the data, while the colored lines are obtained considering only the data in the subset represented in the panel.

Furthermore, playing with the parameters, we confirm that, just like for Model 1, the coefficients $c_n(\sigma)$ in Eq. (S3) clearly depend on the width $\sigma$. These findings suggest that Eq. (S3) truncated to $n$=1 could be used for any JDOS. This is illustrated in Fig. S2 for all our calculated data. The dependence of the coefficients $c_n(\sigma)$ on the width $\sigma$ has been highlighted by splitting the data into 6 groups according to the width of the real JDOS $\sigma$ (computed as the difference between the mean value of the JDOS and the direct gap). This width depends on the dispersion of the bands, hence on the effective mass, and their distribution in energy, as illustrated in Fig. S3. This justifies the use of Eq. (4) in the main text.

## II. COMPARISON OF THE $n_s$-$E_g^d$ MODELS

As mentioned in the main text, different empirical or semi-empirical models have been proposed for the expected inverse relationship between the refractive index $n_s$ and the direct band gap $E_g^d$. A review of such models was recently

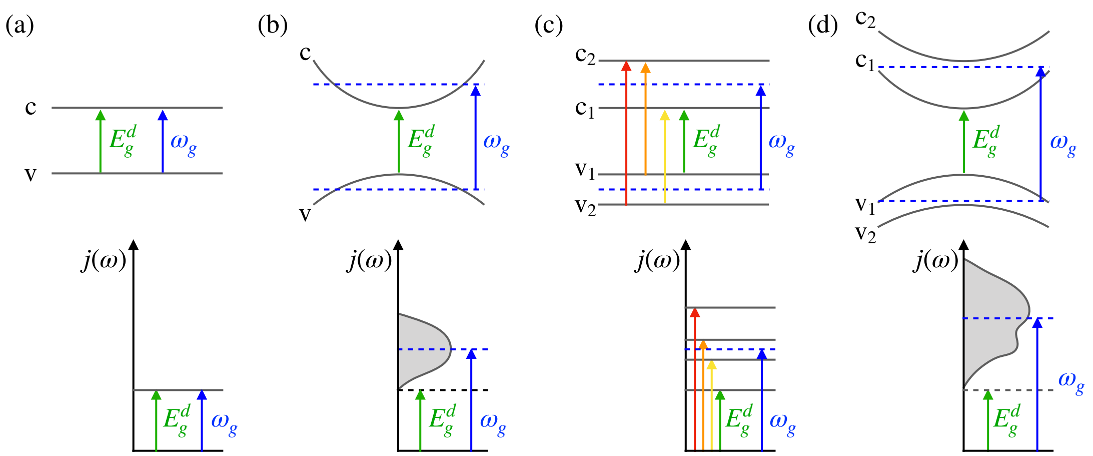


FIG. S3. Schematic illustration of the dependence of the average optical gap $\omega_g$ on the width of the JDOS $j(\omega)$. Starting from a two-state system (a) with flat bands for which $\omega_g$ coincides with the direct band gap $E_g^d$ and $j(\omega)$ is a Dirac peak, the graphs shows how $\omega_g$ is affected by (b) the dispersion of the bands which increases the width of the JDOS, (c) the band distribution in energy when new flat bands are added leading to new Dirac peaks in $j(\omega)$, and (d) the combination of both.

proposed by Tripathy [1]. In Fig. S4, we report the distributions of the absolute errors on the refractive index for various explicit functions of the direct band gap $E_g^d$ compared to the DFPT computed data for the 4040 materials.

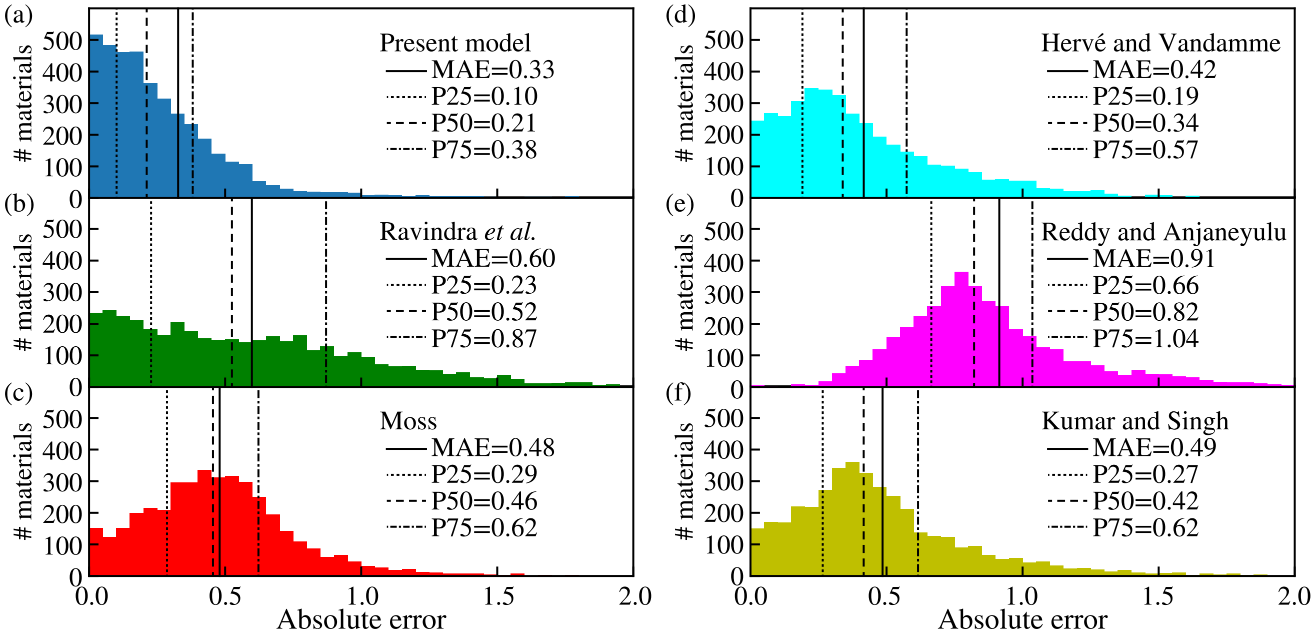


FIG. S4. Distribution of the absolute errors on the refractive index (for various explicit function of the direct band gap $E_g^d$ vs. DFPT) for the 4040 materials. Our model (a) is compared to some well known empirical and semiempirical relations: (b) Ravindra *et al.* [2], (c) Moss [3], (d) Hervé and Vandamme [4], (d) Reddy and Anjaneyulu [5], and (e) Kumar and Singh [6]. For all the models, the mean absolute error (MAE), the 25th, 50th, 75th percentiles (P25, P50, and P75) are indicated.

We consider various descriptors of the distribution of the absolute errors: the mean absolute error (MAE), the 25th, 50th, 75th percentiles (P25, P50, and P75, respectively). All of them indicate that our new model describes the calculated DFPT data better than the previously proposed ones.

## III. COMPARISON WITH THE PENN MODEL

The model presented here can directly be connected to the so-called Penn model in which the static refractive index is given by the following equation:

$$n_s^2 = \varepsilon_{1s} = 1 + \left(\frac{\omega_p}{\omega_g}\right)^2, \tag{S5}$$

where $\omega_p$ is the Drude plasma frequency which is defined through the *f-sum rule*:

$$\int_0^\infty \omega\varepsilon_2(\omega)d\omega = \frac{\pi}{2}\omega_p^2. \tag{S6}$$

Introducing the imaginary part of the dielectric function given by Eq. (A10) of the main text into Eq. (S6) we then obtain:

$$\omega_p^2 = 8\pi K \int_0^\infty \frac{j(\omega)}{\omega} d\omega. \tag{S7}$$

If we now consider the two-state system introduced in the main text whose JDOS is given by $j(\omega) = J\delta(\omega - \omega_g)$, the resulting plasma frequency is simply given by:

$$\omega_p^2 = \frac{8\pi KJ}{\omega_g} = \frac{\omega_{\text{eff}}^3}{\omega_g}. \tag{S8}$$

The two expressions for the static refractive index given by Eq. (A15) of the main text and Eq. (S5) are thus strictly equivalent. Consequently, the model presented in this study is closely related to Penn model. Our model has, however, an important advantage over Penn model for analyzing the data in that the effective frequency $\omega_{\text{eff}}$ is clearly independent of the average optical gap $\omega_g$ (it only depends on the integral of the JDOS $J$ and the average transition probability $K$), while the plasma frequency $\omega_p$ is not.

## IV. AVERAGE TRANSITION PROBABILITY VS. INTEGRAL OF THE JDOS

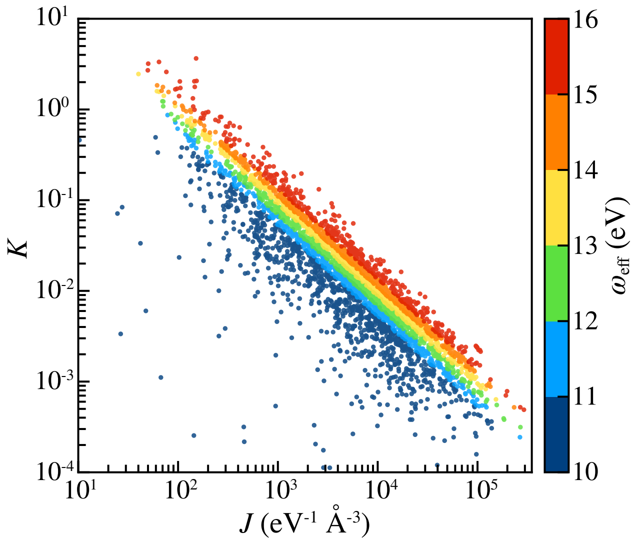


FIG. S5. Calculated values of the average transition probability $K$ and integral of the JDOS $J$ computed up to a frequency $\omega_{\text{max}}$ for the complete dataset of materials. The data are reported as solid circles the color of which refers to the value of $\omega_{\text{eff}}$ as indicated in the color bar.

From Eq. (A13) of the main manuscript we have that $\omega_{\text{eff}}$ is related to the product of the average transition probability $K$ and the integral of the JDOS $J$. In Fig. S5, we show the distribution of all our data points as a function of these two quantities (shown in a logarithmic scale for sake of clarity). The data points have been colored according to $\omega_{\text{eff}}$. Though $K$ is smaller than 1 for the vast majority of materials, both $K$ and $J$ impact the value of $\omega_{\text{eff}}$.

## V. ANALYSIS BY CLASS OF COMPOUNDS

In order to analyze the trend of the data in the different compounds, we separated the oxides (3375 out of 4040) in four classes (see main text): TMOs with empty d shell ($1^{st}$ group) (671 materials); TMOs with partially filled d shell ($2^{nd}$ group) (303); main-group oxides (1520 materials); and lanthanide oxides (747). The result of our analysis is shown in Fig. S6. For each class, an ellipse (in black in the figure) is defined as follows. Its center is located at the average value of $E_g^d$ and $n_s$ for the corresponding distribution. The orientation and lengths of its axes are determined using principal component analysis for the materials which belong to the region with a density larger than 75%.

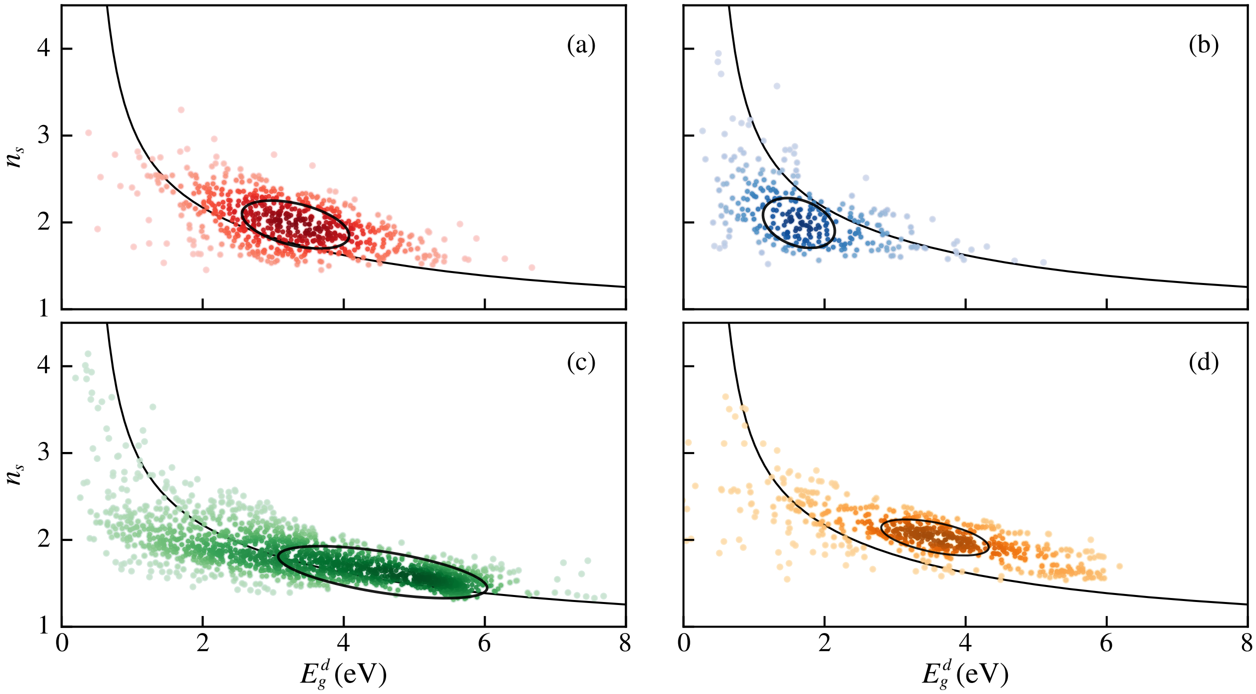


FIG. S6. Static refractive index $n_s$ as a function of the direct band gap $E_g^d$ for the 4 classes of materials: (a) TMOs with empty d shell ($1^{st}$ group) in red, (b) TMOs with partially filled d shell ($2^{nd}$ group) in blue, (c) main-group oxides in green , and (d) lanthanide oxides in orange. The solid line corresponds to Eq. (16) of the main text for the average value of $\omega_{\text{eff}}$=10.75 eV. For each class, the probability density function is computed in the distribution for the refractive index as a function of the band gap via a Kernel-Density Estimation (KDE) using a Gaussian kernel. The darker regions for each class represent the higher value for the distribution density.

## VI. TABLES OF COMPOUNDS

In this section, we provide various tables with the 10 materials with the highest refractive index for a given direct band gap range. In each table the chemical formula, MP identification (mp-id), average refractive index ($n_s$), diagonal components of the refractive index tensor ($n_1$, $n_2$, $n_3$), direct band gap in eV ($E_g^d$), the effective frequency in eV ($\omega_{\text{eff}}$), the average optical gap in eV ($\omega_g$) and the average effective mass of the transitions $\mu$ are shown. The compounds are sorted by the value of the average refractive index. The full list containing the 4040 compounds taken in consideration in this study can be found in the comma-separated values (CSV) file (db.csv).

## VII. IMPORTANCE OF THE EXCHANGE-CORRELATION FUNCTIONAL

It is clear that the exchange-correlation (XC) functional will affect the electronic structure (the band gap and, possibly, the band dispersion) and the optical properties. Here, we analyze how using HSE instead of PBE changes the calculated value of $\omega_g$ for the top materials in the Tables S1-S6. To this end, in Fig. S7, we compare the JDOS $j(\omega)$ and $j(\omega)/\omega^3$ computed with computed with both XC functionals. Obviously, the PBE gaps are smaller than the HSE ones so a scissor $\Delta$ was applied to the PBE electronic structure in order to match the HSE gap. A comparison of the average gap $\omega_g$ computed with PBE+$\Delta_{\text{HSE}}$ and HSE for the selected materials is also shown in Table S7. For each material the value of the $\Delta_{\text{HSE}}$ scissor operator is reported. Looking at the different $\omega_g$ values one can see that there is a small difference considering the two XC functionals, with an absolute error ranging from 0.15 to 1.09 eV.

TABLE S1. List of compounds with $0.0 \leq E_g^d \leq 2.0$ $eV$.

| Formula | mp-id | $n_s$ | $n_1$ | $n_2$ | $n_3$ | $E_g^d$ | $\omega_{\text{eff}}$ | $\omega_g$ | $\mu$ |
|---|---|---|---|---|---|---|---|---|---|
| TePb | mp-19717 | 5.12 | 5.12 | 5.12 | 5.12 | 0.87 | 17.47 | 5.96 | 0.08 |
| $FeS_2$ | mp-1522 | 4.59 | 4.41 | 4.77 | 4.60 | 1.17 | 11.88 | 4.37 | 0.83 |
| $Tl_2S$ | mp-667 | 4.46 | 4.48 | 4.58 | 4.32 | 0.86 | 19.12 | 7.18 | 0.25 |
| SnSe | mp-691 | 4.25 | 4.60 | 4.25 | 3.91 | 0.59 | 7.62 | 2.95 | 0.24 |
| $RuS_2$ | mp-2030 | 4.09 | 4.09 | 4.09 | 4.09 | 0.91 | 13.35 | 5.32 | 0.34 |
| $Sb_2Se_3$ | mp-2160 | 3.90 | 4.30 | 4.28 | 3.10 | 0.80 | 10.76 | 4.45 | 0.47 |
| GeSe | mp-700 | 3.79 | 3.97 | 3.78 | 3.62 | 0.93 | 13.97 | 5.89 | 0.33 |
| $Te_2Mo$ | mp-602 | 3.69 | 4.28 | 4.28 | 2.53 | 1.07 | 10.09 | 4.32 | 0.48 |
| SnS | mp-2231 | 3.68 | 3.85 | 3.58 | 3.60 | 1.07 | 15.37 | 6.61 | 0.24 |
| $Sm_2Te_3$ | mp-684911 | 3.68 | 3.68 | 3.68 | 3.67 | 0.99 | 9.84 | 4.23 | 0.32 |

TABLE S2. List of compounds with $2.0 \leq E_g^d \leq 3.0$ $eV$.

| Formula | mp-id | $n_s$ | $n_1$ | $n_2$ | $n_3$ | $E_g^d$ | $\omega_{\text{eff}}$ | $\omega_g$ | $\mu$ |
|---|---|---|---|---|---|---|---|---|---|
| $TiO_2$ | mp-34688 | 2.61 | 2.65 | 2.65 | 2.52 | 2.35 | 10.77 | 5.99 | 0.94 |
| $YbTe_2$ | mp-1779 | 2.60 | 2.60 | 2.60 | 2.60 | 2.46 | 12.98 | 7.23 | 0.19 |
| $Bi_2O_3$ | mp-23262 | 2.57 | 2.61 | 2.63 | 2.48 | 2.46 | 12.79 | 7.19 | 0.58 |
| $Ti_3PbO_7$ | mp-504427 | 2.57 | 2.60 | 2.59 | 2.51 | 2.32 | 14.01 | 7.90 | 114.11 |
| CaTe | mp-1519 | 2.57 | 2.57 | 2.57 | 2.57 | 2.62 | 11.96 | 6.74 | 0.23 |
| $LiBi_3I_2O_4$ | mp-775430 | 2.56 | 2.62 | 2.62 | 2.44 | 2.25 | 12.40 | 7.00 | 0.55 |
| $B_8O$ | mp-530033 | 2.56 | 2.55 | 2.57 | 2.56 | 2.46 | 18.29 | 10.33 | 1.11 |
| $GeI_2$ | mp-27922 | 2.56 | 2.80 | 2.80 | 2.07 | 2.42 | 11.67 | 6.59 | 1.58 |
| $Bi_4I_2O_5$ | mp-30130 | 2.55 | 2.59 | 2.52 | 2.55 | 2.37 | 11.74 | 6.65 | 0.97 |
| $TiPbO_3$ | mp-20459 | 2.54 | 2.57 | 2.57 | 2.47 | 2.80 | 14.44 | 8.21 | 0.68 |

TABLE S3. List of compounds with $3.0 \leq E_g^d \leq 4.0$ $eV$.

| Formula | mp-id | $n_s$ | $n_1$ | $n_2$ | $n_3$ | $E_g^d$ | $\omega_{\text{eff}}$ | $\omega_g$ | $\mu$ |
|---|---|---|---|---|---|---|---|---|---|
| ZrSO | mp-3519 | 2.78 | 2.78 | 2.78 | 2.78 | 3.01 | 12.71 | 6.73 | 0.70 |
| HfSO | mp-7787 | 2.65 | 2.65 | 2.65 | 2.65 | 3.56 | 13.22 | 7.25 | 0.70 |
| $LiNb_3O_8$ | mp-3368 | 2.39 | 2.45 | 2.38 | 2.34 | 3.00 | 12.15 | 7.25 | 3.62 |
| $Ta_2Pb_2O_7$ | mp-755663 | 2.39 | 2.40 | 2.37 | 2.39 | 3.11 | 15.36 | 9.17 | 5.62 |
| $Nb_2ZnO_6$ | mp-17177 | 2.38 | 2.48 | 2.32 | 2.34 | 3.30 | 13.40 | 8.02 | 3.25 |
| $LaTa_7O_{19}$ | mp-14485 | 2.38 | 2.35 | 2.35 | 2.43 | 3.13 | 13.36 | 8.00 | 2.68 |
| BiClO | mp-22939 | 2.37 | 2.50 | 2.50 | 2.10 | 3.00 | 13.45 | 8.07 | 0.48 |
| $NdTa_7O_{19}$ | mp-14676 | 2.37 | 2.34 | 2.34 | 2.42 | 3.17 | 13.91 | 8.35 | 3.26 |
| $YTa_7O_{19}$ | mp-772036 | 2.36 | 2.34 | 2.34 | 2.42 | 3.16 | 13.81 | 8.31 | 3.45 |
| $BaTiO_3$ | mp-5020 | 2.35 | 2.35 | 2.35 | 2.35 | 2.97 | 12.74 | 7.69 | 1.11 |

TABLE S4. List of compounds with $4.0 \leq E_g^d \leq 5.0\ eV$.

| Formula | mp-id | $n_s$ | $n_1$ | $n_2$ | $n_3$ | $E_g^d$ | $\omega_{\rm eff}$ | $\omega_g$ | $\mu$ |
|---|---|---|---|---|---|---|---|---|---|
| $ZrO_2$ | mp-755089 | 2.26 | 2.28 | 2.20 | 2.30 | 4.15 | 13.78 | 8.59 | 1.35 |
| $ScTaO_4$ | mp-558781 | 2.25 | 2.27 | 2.30 | 2.20 | 4.03 | 13.28 | 8.31 | 1.61 |
| $HfO_2$ | mp-1858 | 2.24 | 2.22 | 2.24 | 2.27 | 4.41 | 15.02 | 9.44 | 1.22 |
| $PrScO_3$ | mp-559756 | 2.22 | 2.24 | 2.23 | 2.19 | 4.26 | 14.05 | 8.90 | 1.15 |
| $Sr_2Zr_7O_{16}$ | mp-770419 | 2.22 | 2.20 | 2.20 | 2.25 | 4.02 | 13.42 | 8.51 | 3.67 |
| $NdScO_3$ | mp-31117 | 2.21 | 2.24 | 2.22 | 2.18 | 4.29 | 13.97 | 8.88 | 1.24 |
| $ThO_2$ | mp-643 | 2.20 | 2.20 | 2.20 | 2.20 | 4.51 | 13.40 | 8.56 | 0.83 |
| $HfO_2$ | mp-775757 | 2.20 | 2.23 | 2.21 | 2.16 | 4.02 | 14.84 | 9.48 | 1.44 |
| $SmScO_3$ | mp-31118 | 2.20 | 2.22 | 2.21 | 2.16 | 4.36 | 13.78 | 8.81 | 1.41 |
| $HfO_2$ | mp-352 | 2.19 | 2.22 | 2.21 | 2.14 | 4.10 | 14.85 | 9.51 | 1.76 |

TABLE S5. List of compounds with $5.0 \leq E_g^d \leq 6.0\ eV$.

| Formula | mp-id | $n_s$ | $n_1$ | $n_2$ | $n_3$ | $E_g^d$ | $\omega_{\rm eff}$ | $\omega_g$ | $\mu$ |
|---|---|---|---|---|---|---|---|---|---|
| BeS | mp-422 | 2.29 | 2.29 | 2.29 | 2.29 | 5.63 | 18.11 | 11.17 | 0.24 |
| $BeSiN_2$ | mp-7913 | 2.13 | 2.16 | 2.14 | 2.11 | 5.30 | 18.77 | 12.30 | 0.39 |
| $LiSi_2N_3$ | mp-5853 | 2.07 | 2.09 | 2.05 | 2.08 | 5.48 | 17.50 | 11.77 | 0.42 |
| DyClO | mp-755323 | 2.07 | 2.09 | 2.09 | 2.02 | 5.17 | 14.68 | 9.88 | 0.45 |
| HoClO | mp-29731 | 2.07 | 2.09 | 2.09 | 2.02 | 5.18 | 14.10 | 9.50 | 0.61 |
| $HfSiO_4$ | mp-4609 | 1.98 | 1.97 | 1.99 | 1.98 | 5.65 | 15.77 | 11.03 | 2.10 |
| $ErBO_3$ | mp-10791 | 1.95 | 1.94 | 1.96 | 1.94 | 5.15 | 15.93 | 11.32 | 2.68 |
| $Pr_3Si_2ClO_8$ | mp-554826 | 1.93 | 1.93 | 1.93 | 1.93 | 5.15 | 14.79 | 10.56 | 1.25 |
| $Nd_2Be_2SiO_7$ | mp-9077 | 1.92 | 1.89 | 1.93 | 1.93 | 5.03 | 15.86 | 11.41 | 0.64 |
| $Y_2Be_2SiO_7$ | mp-6655 | 1.90 | 1.87 | 1.91 | 1.91 | 5.19 | 15.57 | 11.31 | 0.63 |

TABLE S6. List of compounds with $6.0 \leq E_g^d \leq 7.0\ eV$.

| Formula | mp-id | $n_s$ | $n_1$ | $n_2$ | $n_3$ | $E_g^d$ | $\omega_{\rm eff}$ | $\omega_g$ | $\mu$ |
|---|---|---|---|---|---|---|---|---|---|
| $BeAl_2O_4$ | mp-3081 | 1.78 | 1.78 | 1.78 | 1.78 | 6.12 | 18.71 | 14.45 | 0.37 |
| $MgAlBO_4$ | mp-8376 | 1.72 | 1.72 | 1.72 | 1.72 | 6.23 | 17.76 | 14.20 | 0.42 |
| LiCl | mp-22905 | 1.72 | 1.72 | 1.72 | 1.72 | 6.25 | 15.92 | 12.75 | 0.38 |
| $LaF_3$ | mp-905 | 1.70 | 1.70 | 1.70 | 1.70 | 6.04 | 10.20 | 8.24 | 9.19 |
| $NaPr_2S_2O_8F_3$ | mp-560673 | 1.70 | 1.70 | 1.71 | 1.68 | 6.18 | 14.97 | 12.13 | 6.05 |
| $CaB_2O_4$ | mp-8056 | 1.69 | 1.73 | 1.71 | 1.64 | 6.09 | 15.18 | 12.31 | 0.60 |
| $Al_6B_5O_15F_3$ | mp-6738 | 1.68 | 1.68 | 1.68 | 1.67 | 6.17 | 17.08 | 14.03 | 0.53 |
| $BaBePO_4F$ | mp-754604 | 1.67 | 1.67 | 1.67 | 1.67 | 6.24 | 15.22 | 12.52 | 0.47 |
| $SiO_2$ | mp-549166 | 1.65 | 1.82 | 1.57 | 1.57 | 6.00 | 16.26 | 13.53 | 0.47 |
| $LiB_3O_5$ | mp-3660 | 1.62 | 1.63 | 1.64 | 1.60 | 6.35 | 16.13 | 13.70 | 1.02 |

TABLE S7. Comparison of the $\omega_g$ values (in eV) computed considering PBE+$\Delta_{\mathrm{HSE}}$ and HSE for the top materials in the Tables S1-S6. For each material also the value of the scissor operator $\Delta_{\mathrm{HSE}}$ (in eV) is reported.

| Formula | MP-id | $\Delta_{\mathrm{HSE}}$ | $\omega_g$ (PBE+$\Delta_{\mathrm{HSE}}$) | $\omega_g$ (HSE) |
|---|---|---|---|---|
| TePb | mp-19717 | 0.54 | 7.09 | 6.00 |
| $TiO_2$ | mp-34688 | 1.57 | 7.73 | 8.00 |
| ZrSO | mp-3519 | 1.30 | 8.24 | 8.39 |
| $ZrO_2$ | mp-755089 | 1.84 | 10.52 | 10.75 |
| BeS | mp-422 | 1.26 | 12.41 | 12.64 |
| $BeAl_2O_4$ | mp-3081 | 2.25 | 16.59 | 16.79 |

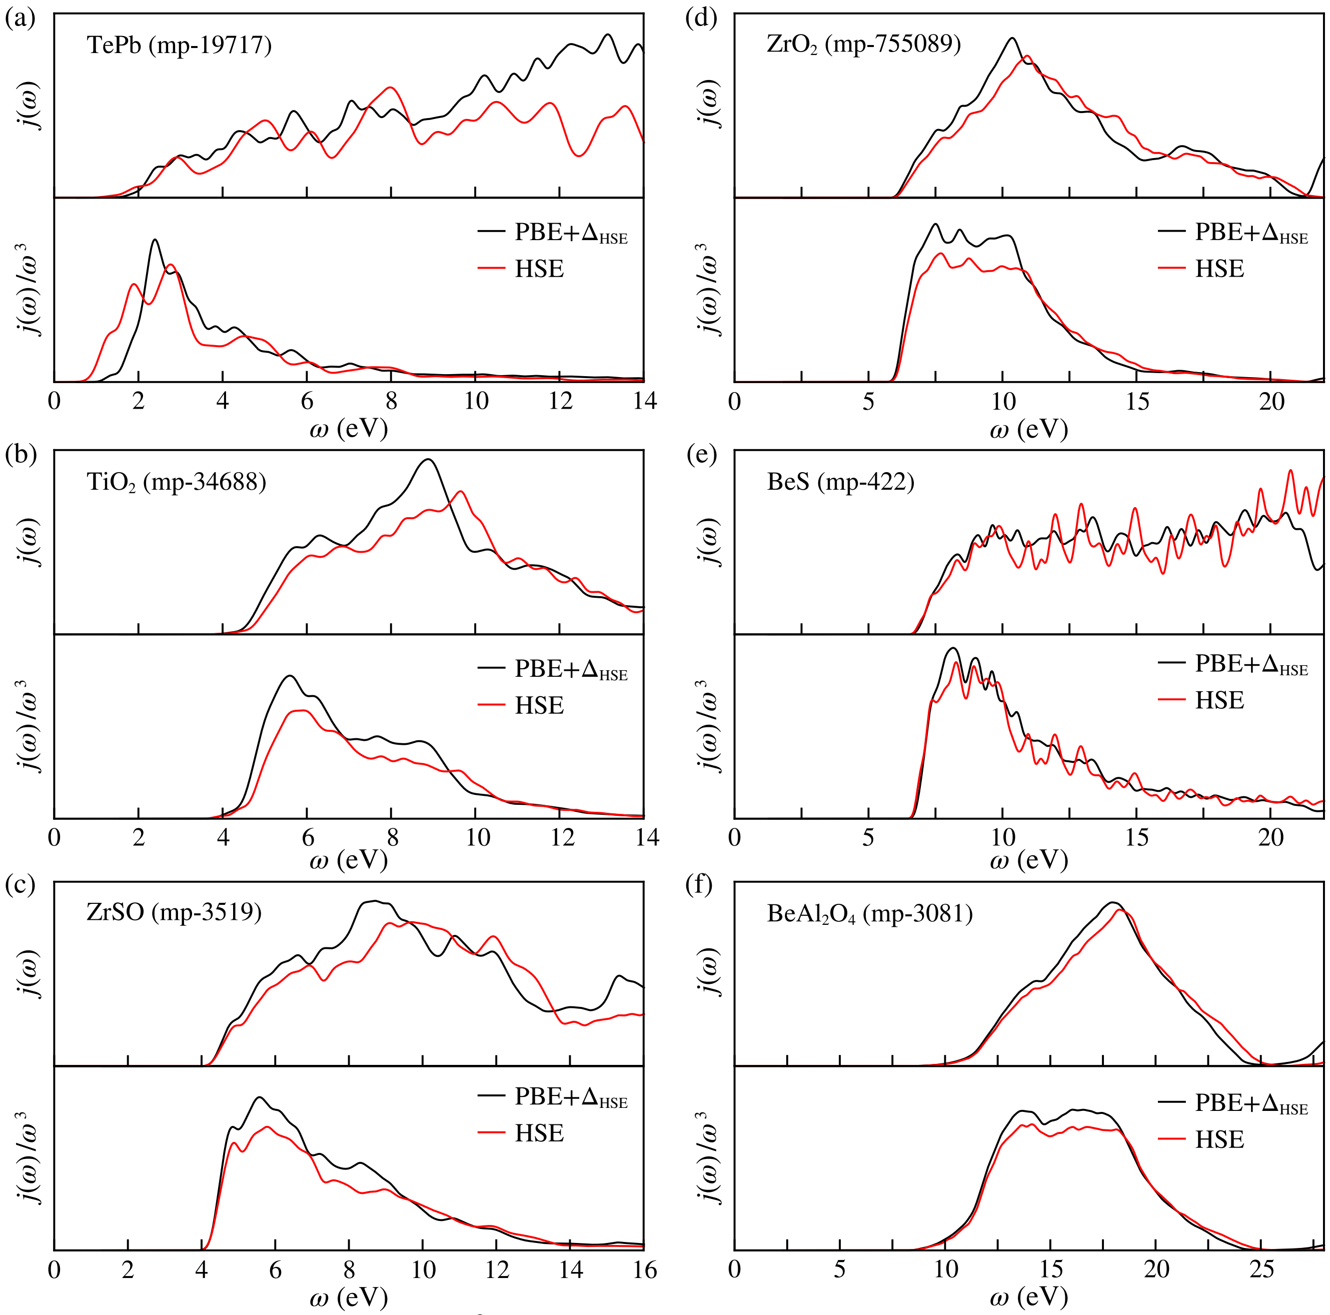


FIG. S7. Optical functions $j(\omega)$ and $j(\omega)/\omega^3$ computed with PBE+$\Delta_{\mathrm{HSE}}$ and HSE for the top materials in the Tables S1-S6.

[1] S. Tripathy, Opt. Mater. **46**, 240 (2015).
[2] N. M. Ravindra, S. Auluck, and V. K. Srivastava, Phys. Status Solidi B **93**, K155 (1979).
[3] T. S. Moss, Phys. Status Solidi B **131**, 415 (1985).
[4] P. Hervé and L. Vandamme, Infrared Phys. Technol. **35**, 609 (1994).
[5] R. R. Reddy and S. Anjaneyulu, Phys. Status Solidi B **174**, K91 (1992).
[6] V. Kumar and J. Singh, Indian J. Pure Appl. Phys. **48**, 571 (2010).
